# Supplementary material for: Switching nonparametric regression models for multi-curve data
Source: arXiv:1504.02813 ancillary file (2017-09-13)
Supplement: Supplementary file 1 [file DeSouza-etal-ArXiv-Supplement.pdf]

# Switching nonparametric regression models for multi-curve data

## Supplementary Material

Camila P. E. de Souza, Nancy E. Heckman and Helena Xu

### 1 Updating $\mathbf{V}$ in the EM algorithm

To update our estimate of  $\mathbf{V}$ , we maximize Equation (8) in Section 3.2 of the main paper as a function of parameters in  $\mathbf{V}$ , that is, we minimize

$$\tilde{S} = \sum_{k=1}^N \sum_{\text{all } \mathbf{s}'\text{'s}} p_k(\mathbf{s})^{(c)} \left[ (\mathbf{y}_k - f_{\mathbf{s}}(\mathbf{x}))^T \mathbf{V}_{\mathbf{s}}^{-1} (\mathbf{y}_k - f_{\mathbf{s}}(\mathbf{x})) + \log |\mathbf{V}_{\mathbf{s}}| \right].$$

*Updating  $\mathbf{V}$  for unrestricted  $\mathbf{V}$ , with no dependence on  $\mathbf{z}$ .*

We rewrite  $\mathbf{V}_{\mathbf{s}} = \mathbf{V}$  and

$$\begin{aligned} \tilde{S} &= N \log |\mathbf{V}| + \sum_{k=1}^N \sum_{\text{all } \mathbf{s}'\text{'s}} p_k(\mathbf{s})^{(c)} \left[ (\mathbf{y}_k - f_{\mathbf{s}}(\mathbf{x}))^T \mathbf{V}^{-1} (\mathbf{y}_k - f_{\mathbf{s}}(\mathbf{x})) \right] \\ &= N \log |\mathbf{V}| + \text{tr} \left[ \mathbf{V}^{-1} \sum_{k=1}^N \sum_{\text{all } \mathbf{s}'\text{'s}} p_k(\mathbf{s})^{(c)} (\mathbf{y}_k - f_{\mathbf{s}}(\mathbf{x})) (\mathbf{y}_k - f_{\mathbf{s}}(\mathbf{x}))^T \right] \end{aligned}$$

and apply Result 4.10 of Johnson and Wichern (2008) to  $\exp(-\tilde{S})$  to obtain the expression for  $\hat{\mathbf{V}}$  in Equation (11) of the main paper.

*Updating  $\mathbf{V}$  generated by the homogeneous random intercept model.*

Note that  $\mathbf{V}_{\mathbf{s}} = \mathbf{V} = \sigma^2(\mathbf{I} + d\mathbf{1}\mathbf{1}^T)$  as in Equation (3) of the main paper. We can calculate the determinant and inverse of  $\mathbf{V}$  using the so-called dimension-reduction formulae (see Section 2.2.3 of Demidenko, 2004) as follows:

$$|\mathbf{V}| = \sigma^{2n} |\mathbf{I} + d\mathbf{1}\mathbf{1}^T| = \sigma^{2n} (1 + d\mathbf{1}^T \mathbf{1}) = \sigma^{2n} (1 + nd),$$

and

$$\mathbf{V}^{-1} = \frac{1}{\sigma^2} \left( \mathbf{I} - \frac{d}{1 + nd} \mathbf{1}\mathbf{1}^T \right).$$

Thus, we can rewrite  $\tilde{S}$  as

$$\begin{aligned} \tilde{S} &= N \log(1 + nd) + Nn \log \sigma^2 \\ &\quad + \frac{1}{\sigma^2} \sum_{k=1}^N \sum_{\text{all } \mathbf{s}'\text{'s}} p_k(\mathbf{s})^{(c)} \|\mathbf{y}_k - f_{\mathbf{s}}(\mathbf{x})\|^2 \\ &\quad - \frac{d}{\sigma^2(1 + nd)} \sum_{k=1}^N \sum_{\text{all } \mathbf{s}'\text{'s}} p_k(\mathbf{s})^{(c)} [(\mathbf{y}_k - f_{\mathbf{s}}(\mathbf{x}))^T \mathbf{1}]^2. \end{aligned}$$

We minimize  $\tilde{S}$  first with respect to  $d$ , yielding  $\hat{d}$  as in Equation (13) of the main paper. Replacing  $d$  by  $\hat{d}$  in  $\tilde{S}$  and then minimizing with respect to  $\sigma^2$ , we obtain Equation (12) of the main paper.

*Updating  $\mathbf{V}$  generated by the non-homogeneous random intercept model,  $J = 2$  states.*

Note that in this model, the covariance matrix  $\mathbf{V}_{\mathbf{s}}$  depends on  $\mathbf{s}$ , as given in Equation (4) of the main paper. We maximize  $\tilde{S}$  as a function of  $\sigma^2$ ,  $d_1$  and  $d_2$  numerically, after first writing  $\mathbf{V}_{\mathbf{s}}^{-1}$  as

$$\sigma^2 \mathbf{V}_{\mathbf{s}}^{-1} = (a_{\mathbf{s},d_1,d_2})\mathbf{I} + (b_{\mathbf{s},d_1,d_2})\mathbf{1}\mathbf{1}^T + (c_{\mathbf{s},d_1,d_2})\mathbf{1}\mathbf{1}_{\mathbf{s}}^T + (f_{\mathbf{s},d_1,d_2})\mathbf{1}_{\mathbf{s}}\mathbf{1}^T + (g_{\mathbf{s},d_1,d_2})\mathbf{1}_{\mathbf{s}}\mathbf{1}_{\mathbf{s}}^T$$

where  $a, b, c, f$ , and  $g$  can be easily found for specific values of  $\mathbf{s}$  by solving the linear system gotten by writing  $(\mathbf{V}_{\mathbf{s}})^{-1} \times \mathbf{V}_{\mathbf{s}} = \mathbf{I}$ . We maximize  $\tilde{S}$  with respect to  $\sigma^2$ ,  $d_1$  and  $d_2$  by first fixing  $d_1$  and  $d_2$ , then calculating  $\hat{\sigma}^2$ . We then fix  $\hat{\sigma}^2$  and calculate  $\hat{d}_1$  and  $\hat{d}_2$ .

## 2 Calculation details: standard errors for Markov $z_{ik}$ 's

We can show that the  $3 \times 3$  matrix  $E_{\alpha}(\mathcal{L}'_2(\alpha)\mathcal{L}'_2(\alpha)^T | \mathbf{y}^R)$  from Section 4.2 of the main paper evaluated at  $\alpha = \hat{\alpha}$  with  $\gamma = \hat{\gamma}$  is symmetric with diagonal elements

$$\sum_{k=1}^N \sum_{\text{all } \mathbf{s}'\mathbf{s}} \hat{p}_k(\mathbf{s}) \left( \frac{I(s_1=1)}{\hat{\pi}_1} - \frac{I(s_1=2)}{(1-\hat{\pi}_1)} \right)^2 - \sum_{k=1}^N \left[ \sum_{\text{all } \mathbf{s}'\mathbf{s}} \hat{p}_k(\mathbf{s}) \left( \frac{I(s_1=1)}{\hat{\pi}_1} - \frac{I(s_1=2)}{(1-\hat{\pi}_1)} \right) \right]^2,$$

$$\sum_{k=1}^N \sum_{\text{all } \mathbf{s}'\mathbf{s}} \hat{p}_k(\mathbf{s}) \left( \frac{n_{\mathbf{s},12}}{\hat{a}_{12}} - \frac{n_{\mathbf{s},11}}{(1-\hat{a}_{12})} \right)^2 - \sum_{k=1}^N \left[ \sum_{\text{all } \mathbf{s}'\mathbf{s}} \hat{p}_k(\mathbf{s}) \left( \frac{n_{\mathbf{s},12}}{\hat{a}_{12}} - \frac{n_{\mathbf{s},11}}{(1-\hat{a}_{12})} \right) \right]^2$$

and

$$\sum_{k=1}^N \sum_{\text{all } \mathbf{s}'\mathbf{s}} \hat{p}_k(\mathbf{s}) \left( \frac{n_{\mathbf{s},21}}{\hat{a}_{21}} - \frac{n_{\mathbf{s},22}}{(1-\hat{a}_{21})} \right)^2 - \sum_{k=1}^N \left[ \sum_{\text{all } \mathbf{s}'\mathbf{s}} \hat{p}_k(\mathbf{s}) \left( \frac{n_{\mathbf{s},21}}{\hat{a}_{21}} - \frac{n_{\mathbf{s},22}}{(1-\hat{a}_{21})} \right) \right]^2.$$

The [1,2], [1,3] and [2,3] off diagonal elements are

$$\begin{aligned} & \sum_{k=1}^N \sum_{\text{all } \mathbf{s}'\mathbf{s}} \hat{p}_k(\mathbf{s}) \left( \frac{I(s_1=1)}{\hat{\pi}_1} - \frac{I(s_1=2)}{(1-\hat{\pi}_1)} \right) \left( \frac{n_{\mathbf{s},12}}{\hat{a}_{12}} - \frac{n_{\mathbf{s},11}}{(1-\hat{a}_{12})} \right) \\ & - \sum_{k=1}^N \left[ \sum_{\text{all } \mathbf{s}'\mathbf{s}} \hat{p}_k(\mathbf{s}) \left( \frac{I(s_1=1)}{\hat{\pi}_1} - \frac{I(s_1=2)}{(1-\hat{\pi}_1)} \right) \times \sum_{\text{all } \mathbf{s}'\mathbf{s}} \hat{p}_k(\mathbf{s}) \left( \frac{n_{\mathbf{s},12}}{\hat{a}_{12}} - \frac{n_{\mathbf{s},11}}{(1-\hat{a}_{12})} \right) \right], \\ & \sum_{k=1}^N \sum_{\text{all } \mathbf{s}'\mathbf{s}} \hat{p}_k(\mathbf{s}) \left( \frac{I(s_1=1)}{\hat{\pi}_1} - \frac{I(s_1=2)}{(1-\hat{\pi}_1)} \right) \left( \frac{n_{\mathbf{s},21}}{\hat{a}_{21}} - \frac{n_{\mathbf{s},22}}{(1-\hat{a}_{21})} \right) \\ & - \sum_{k=1}^N \left[ \sum_{\text{all } \mathbf{s}'\mathbf{s}} \hat{p}_k(\mathbf{s}) \left( \frac{I(s_1=1)}{\hat{\pi}_1} - \frac{I(s_1=2)}{(1-\hat{\pi}_1)} \right) \times \sum_{\text{all } \mathbf{s}'\mathbf{s}} \hat{p}_k(\mathbf{s}) \left( \frac{n_{\mathbf{s},21}}{\hat{a}_{21}} - \frac{n_{\mathbf{s},22}}{(1-\hat{a}_{21})} \right) \right] \end{aligned}$$

and

$$\sum_{k=1}^N \sum_{\text{all } \mathbf{s}'\mathbf{s}} \hat{p}_k(\mathbf{s}) \left( \frac{n_{\mathbf{s},12}}{\hat{a}_{12}} - \frac{n_{\mathbf{s},11}}{(1-\hat{a}_{12})} \right) \left( \frac{n_{\mathbf{s},21}}{\hat{a}_{21}} - \frac{n_{\mathbf{s},22}}{(1-\hat{a}_{21})} \right)$$

$$- \sum_{k=1}^N \left[ \sum_{\text{all } \mathbf{s}'\mathbf{s}} \hat{p}_k(\mathbf{s}) \left( \frac{n_{\mathbf{s},12}}{\hat{a}_{12}} - \frac{n_{\mathbf{s},11}}{(1 - \hat{a}_{12})} \right) \times \sum_{\text{all } \mathbf{s}'\mathbf{s}} \hat{p}_k(\mathbf{s}) \left( \frac{n_{\mathbf{s},21}}{\hat{a}_{21}} - \frac{n_{\mathbf{s},22}}{(1 - \hat{a}_{21})} \right) \right],$$

respectively.

## References

Demidenko, E. (2004), *Mixed Models: Theory and Applications*, John Wiley & Sons.

Johnson, R. A. and Wichern, D. W. (2008), *Applied Multivariate Statistical Analysis*, 6th Ed., Pearson.
